# Supplementary material for: Auxiliary Learning for Deep Multi-task Learning
Source: arXiv:1909.02214 source file (2019-11-28)
Supplement: Supplementary file 1 [file supplementary.tex]

\section{Appendix}  \label{sec:appendix}

\subsection{Extension to multi-task} \label{appendix:multi-task}
To train a multi-task learning system, firstly we need to get a large dataset with the mapping from a single input space $\mathcal{X}$ to multiple labels $\mathcal{\{Y\}}^{t}_{t \in \{T\}}$ , i.i.d. ${\{x_{i},y_{i}^{1},\cdots,y_{i}^{T}\}_{i \in \{N\}}}$, where $T$ is the number of the tasks and $N$ is the number of the data samples. 
The MTL network $\mathcal{F}$ consists of a single shared parameter space $\bm{\theta}^{sh}$ and $T$ sets of task-specific parameters $\bm{\theta}^{t}$. Here we denote the loss function for task $t$ as $\mathcal{L}^t(\cdot)$ to describe the difference between the output of $\mathcal{F}$ for task $t$: $f^{t}(\mathcal{X};\bm{\theta}^{\mathcal{B}},\bm{\theta}^{t})$, and the ground truth label: $\mathcal{\{Y\}}^{t}$. Therefore, we formulate the final objective function for a hard parameter sharing network as follows:
\begin{equation}
\label{eq:mtl}
    \mathop {\min }\limits_{\{\bm{\theta}^{sh},\bm{\theta}^{1},\cdots,\bm{\theta}^{T}\}}\sum_{t=1}^{T} \alpha^{t} \mathcal{L}^t(f^{t}(\mathcal{X};\bm{\theta}^{sh},\bm{\theta}^{t}),\mathcal{\{Y\}}^{t}),
\end{equation}
where $\alpha^{t}$ is a combination coefficient for the $t$-th task. In this work, we do not focus on adjusting the $\alpha^{t}$ to boost the performance, so we set the $\alpha^{t}=1$ to all cases to simplify the basic objective function to $
    \mathop {\min }\limits_{\{\bm{\theta}^{sh},\bm{\theta}^{1},\cdots,\bm{\theta}^{T}\}}\sum_{t=1}^{T} \mathcal{L}^t(f^{t}(\mathcal{X};\bm{\theta}^{sh},\bm{\theta}^{t}),\mathcal{\{Y\}}^{t})$.

The basic structure of an auxiliary module for task $t$ is the same as shown in the main paper, and we can extend the objective function (\ie, Eq. (2)) in the main paper to multi-task case as follows:
\begin{equation}
  \begin{aligned}
        & \mathop {\min }\limits_{\{\bm{\theta}^{sh},\bm{\theta}^{1},\cdots,\bm{\theta}^{T},\bm{\theta}_{a}^{1},\cdots,\bm{\theta}_{a}^{T}\}}(\sum_{t=1}^{T} \mathcal{L}^t(f^{t}(\mathcal{X};\bm{\theta}^{sh},\bm{\theta}^{t}),\mathcal{\{Y\}}^{t})  \\
        & +\sum_{t=1}^{T}\mathcal{L}^t_{aux}(\mathcal{A}^{t}(\bm{O}_{1},\cdots,\bm{O}_{L};\bm{\theta}^{sh},\bm{\theta}_{a}^{t}),\mathcal{\{Y\}}^{t})),
    \end{aligned}
\end{equation}
where $\btheta_{a}^{t}$ and $\mathcal{L}^t_{aux}(\cdot)$ represent the adaptor parameters and the auxiliary loss for the $t$-th task, respectively.

To extend the search policy to the multi-task case, as described in the main paper, we enlarge the output length of the controller to $T$ times as many as a single task, and follow the order in Fig. \ref{fig:nas1}. We have reserved the possibility of association between different tasks in the search space, for example, for the $l$-$th$ cell in task $t$, it can choose the output of task $1$ to task $t-1$ in the first $l-1$ cells as input. The auxiliary module $\mathcal{A}$ can learn a heretical relationships among all tasks. We show the search results of a sampled structure, which has the highest reward score on the validation set in Fig. \ref{fig:nas_de}.
\begin{figure*}[htb]
  \centering
  \includegraphics[width=1\textwidth]{./images/nas.pdf}
  \caption{(a) Auxiliary structure search space for the multi-task learning. (b) Controller output for generating a single cell for the $l$-$th$ auxiliary cell of task $t$, $\mathcal{A}_l^t$. (c) The order of generating the whole auxiliary module recursively among different tasks. }
  \label{fig:nas1}
\end{figure*}

\begin{figure*}[htb]
  \centering
  \includegraphics[width=0.9\textwidth]{./images/nas_strucutre.pdf}
  \caption{The auxiliary modules sampled by the reinforcement learning. We show the detailed structure used in the multi-task experiments for depth prediction and semantic segmentation.}
  \label{fig:nas_de}
\end{figure*}

\subsection{Training details} \label{appendix:training}
In this section, we will introduce the training setups for the experiments. All the experiments are implemented in pytorch.
\subsection{Semantic segmentation}
As for the single task of semantic segmentation, we use the open source implementation \citep{zhou2017scene}, and follow their settings. We set the initial learning rate as $0.02$ and weight decay as $0.0001$ by default, the input image is resized to the length randomly chosen from the set {$300$, $375$, $450$, $525$, $600$} due to that the images are of various sizes on ADE$20$K. The batch size is $8$ and we also synchronize the mean and standard-deviation of BN cross multiple GPUs. We train all the experiments for $20$ epochs. 

\subsubsection{Multi-task learning}
Common data augmentation is employed with the random flip, random reshape (from $0.5$ to $2.1$) and random crop with the training size $385 \times 385$. The ground truth of depth should be normalized with the scale of random reshape. The batch size is $12$ for all experiments.
In the Sec.4.2.2, we verify our proposed method on the \emph{NYUD-v2} dataset. We train the \emph{single} task baseline and the \emph{joint} baseline for $30k$ iterations with the initial learning rate of $0.01$ and weight decay of $0.0001$. The learning rate is multiplied by $(1-\frac{iter}{max-iter})^{0.9}$. For the \emph{prior} training strategy, we initialize the network with the single task baseline, and then jointly train two tasks with learning rate $0.001$ for $30k$ iterations with the same learning rate schedule. To make a fair comparison, for adding a single auxiliary module, we follow the same training setting with \emph{prior}. And when adding auxiliary modules supervised by two tasks, we follow the training setups of the \emph{joint} baseline. 
In other sections, the models are pretrained on \emph{NYUD-v2-expansion} for $40k$ iterations with initial learning rate of $0.01$, and then fine tune on the \emph{NYUD-v2} with a fixed learning rate of $0.00001$ for $10k$ iterations.
On the \emph{SUNRGBD} dataset, the models are trained for $80k$ iterations with the initial learning rate of $0.01$ both with and without auxiliary modules. 

\subsection{Visualization results}
In this section, we show some visualization results on \textsl{NYUD-v2} and \textsl{SUNRGBD}. The multi-task system can generate multiple outputs in one forward pass.
\begin{figure*}[htb]
  \centering
  \includegraphics[width=0.9\textwidth]{./images/vis.pdf}
  \caption{\textbf{Visualization Results on NYUD-v2} (a) Input image. (b) Predicted depth results. (c) Ground truth depth results. (d) Predicted semantic segmentation results. (e) Ground truth semantic segmentation results. }
  \label{fig:vis}
\end{figure*}

\begin{figure*}[htb]
  \centering
  \includegraphics[width=0.9\textwidth]{./images/vis_sunrgbd.pdf}
  \caption{\textbf{Visualization Results on SUNRGBD} (a) Input image. (b) Predicted surface normal. (c) Ground truth surface normal. (d) Predicted semantic segmentation results. (e) Ground truth semantic segmentation results. (f) Predicted depth results. (e) Ground truth depth results.}
  \label{fig:vis_sun}
\end{figure*}
